# Supplementary material for: What Was Your Prompt? A Remote Keylogging Attack on AI Assistants
Source: arXiv:2403.09751 source file (2024-03-14)
Supplement: Supplementary file 1 [file appendix_examples.tex]

\begin{figure}
\begin{tcolorbox}[title = Additional Examples]

\setstretch{0.9}

\underline{$\phi: 0.64$ \hspace{1em} ROUGE-1: $0.93$
\hspace{1em} Edit Distance: $0.04$}
\vspace{.5em}\\
\small
As an AI language model, I don't have access to the latest \textcolor{black}{\textbf{trade}} statistics,
\vspace{.3em}

As an AI language model, I don't have access to the latest \textcolor{BrickRed}{\textbf{crime}} statistics,
\normalsize \newline
We can see that the comes out to one word, and the scores are effected of course, mainly the $\phi:$. This raises up some points:
\begin{enumerate}
\item We should look at \textbf{both} $\phi:$ of the Sentence-Transformer and ROUGE1 in order to fully evaluate the model's performance.
\item Sometimes, we are just limited, due to the hardness of this problem. Unless the model would have memorized, with no different heuristic we are limited.
\end{enumerate}

\noindent\makebox[\linewidth]{\rule{1.1\columnwidth}{0.4pt}}

The model is good at identifying patterns and have truly learned the meaning of each token-length. \newline
1. Promotion of \textcolor{black}{\textbf{Environmentalism}}: Music festivals have long... \newline
1. Investing in \textcolor{black}{\textbf{multiculturalism}}: Music festivals have been... \newline 
Environmentalism is tokenized as Environmental+ism and same for multiculturalism. And the model got the pattern right.
\noindent\makebox[\linewidth]{\rule{1.1\columnwidth}{0.4pt}}

\end{tcolorbox}
\vspace{-1em}
 \end{figure}

% \noindent\begin{minipage}{\textwidth}
% \captionof{figure}{A box}\label{box}
% \end{minipage}
